# Supplementary material for: HEnRY: A Multi-Agent System Framework for Multi-Domain Contexts
Source: arXiv:2410.12720 source file (2024-10-16)
Supplement: Supplementary file 1 [file a2.tex]

\subsection{HENRY Project Principles}

The HENRY project is also based on some principles defined in this work.

\begin{itemize}

    \item[] \textbf{The modularity principle}: Each MAS instance acts as a unique touchpoint for the human user. Each domain is composed of the same type of agents but with different implementations. This abstraction simplify the management of the MAS.
    
    \item[] \textbf{The omnichannel principle}: A user can access the system through various channels (e.g., web application, mobile application). This decoupling is achieved by instantiating an agent that acts as a user digital twin connected to the MAS. Thus, the user experiences the assistant as an AI companion through their preferred channel, while the user (or more precisely, their digital twin) functions as an agent within the MAS, acting as a leader.
    
    \item[] \textbf{Knowledge sharing principle}: The leader agents possess foundational knowledge of the company, which they use to interact with two types of agents: \textit{facilitators} (for synchronous, in-depth domain knowledge) and \textit{mediators} (for asynchronous requests). These interactions engage various domain agents to provide explanations about knowledge bases, achieve goals, or complete tasks. In this way, the leaders can assist users by seeking domain-specific help for knowledge or tasks from the relevant domains.
    
    \item[] \textbf{Multi-Domain interface principle}: Each domain has an agent (or a group of agents) that acts as an interface between the MAS and the company's IT system. This setup allows for:
    \begin{itemize}
    \item \textbf{Easy integration}: Simplifies the process of plugging a domain into the system through a general interface, facilitating straightforward extensions of the MAS. Domain agents function as domain service providers in the MAS;
    \item \textbf{Human interaction}: Allows domain agents to request assistance from humans or require actions, ensuring easy inclusion of human in the loop;
    \item \textbf{Business unit mapping}: Enables agents to align with the appropriate business unit of the company, streamlining the mapping process;
    \item \textbf{Ownership separation}: Ensures each domain remains autonomous, capable of announcing new services or managing its own evolution. Additionally, domain agents can control the frequency of resource requests from other agents to align with the domain's timing dynamics;
    \item \textbf{Expert maintenance}: Allows software development and maintenance to be managed by expert teams within each domain, ensuring the system's functionality and upkeep.
    \end{itemize}
\end{itemize}
